# Supplementary material for: Chemical Potential Calculations in Non-Homogeneous Liquids
Source: arXiv:1804.03477 ancillary file (2018-05-08)
Supplement: Supplementary file 1 [file SIjcp_22_2.pdf]

# Supplementary Material for: Chemical Potential Calculations in Non-Homogeneous Liquids

C. Perego,[1,2,3,a)] O. Valsson,[1,2,3] and M. Parrinello[2,3]

[1)] *Department of Polymer Theory, Max-Planck Institute for Polymer Research, Ackermannweg 10, D-55128 Mainz (Germany)*

[2)] *Department of Chemistry and Applied Biosciences, ETH Zurich, c/o USI Campus, Via Giuseppe Buffi 13, CH-6900 Lugano (Switzerland)*

[3)] *Università della Svizzera italiana, Institute of Computational Science, National Center for Computational Design and Discovery of Novel Materials MARVEL, Università della Svizzera italiana, Via Giuseppe Buffi 13, CH-6900 Lugano (Switzerland)*

[a)] perego@mpip-mainz.mpg.de

# I. PREVENTION OF SYSTEMATIC ERRORS IN CHEMICAL POTENTIAL CALCULATIONS

The results reported in Fig. 3 of the main text show that there is a deviation between the metadynamics chemical potential estimate and the Widom one, that we motivate with a systematic error, which is not present in our metadynamics method. The figure shows that the $\mu^{\text{ex}}$ value resulting from a more extensive metadynamic calculation, with $M = 512$ insertion points, is compatible with the other metadynamics estimates, but not with the Widom one. This suggests that our estimate is robust, independently from the number of insertion points. In Fig. 1 we compare the convergence of $\mu^{\text{ex}}$ calculated by three different Widom computations, respectively with $M_{\text{W}} = 4000$, 27000 and 512000 insertions per step, with the result of the metadynamics calculations reported in the main text (type I and II with $M = 64$, and type I with $M = 512$). The final chemical potential estimates are reported in Tab. I. The results underline the deviation between Widom and metadynamics computations. Moreover we stress the fact that when a very large number of insertions per step is employed ($M_{\text{W}} = 512000$) the Widom's estimate tends to reduce the gap with the metadynamics ones. That is because a larger number of random insertions attains a better sampling of the low insertion energy tail, resulting in a smaller systematic error.

| Method | $\mu^{\text{ex}}$ $[\epsilon]$ |
|---|---|
| Widom $M_{\text{W}} = 4000$ | $-0.972 \pm 0.024$ |
| Widom $M_{\text{W}} = 27000$ | $-0.970 \pm 0.012$ |
| Widom $M_{\text{W}} = 512000$ | $-0.980 \pm 0.006$ |
| Meta I $M = 64$ | $-0.992 \pm 0.014$ |
| Meta II $M = 64$ | $-0.992 \pm 0.015$ |
| Meta I $M = 512$ | $-0.989 \pm 0.010$ |

TABLE I. $\mu^{\text{ex}}$ estimates obtained for the $N = 920$ system. The first column indicates the calculation method. The chemical potential is computed after $5 \times 10^5 \Delta\tau$ steps, the uncertainty corresponds to the statistical error of the estimate, calculated combining bootstrap and block averaging.

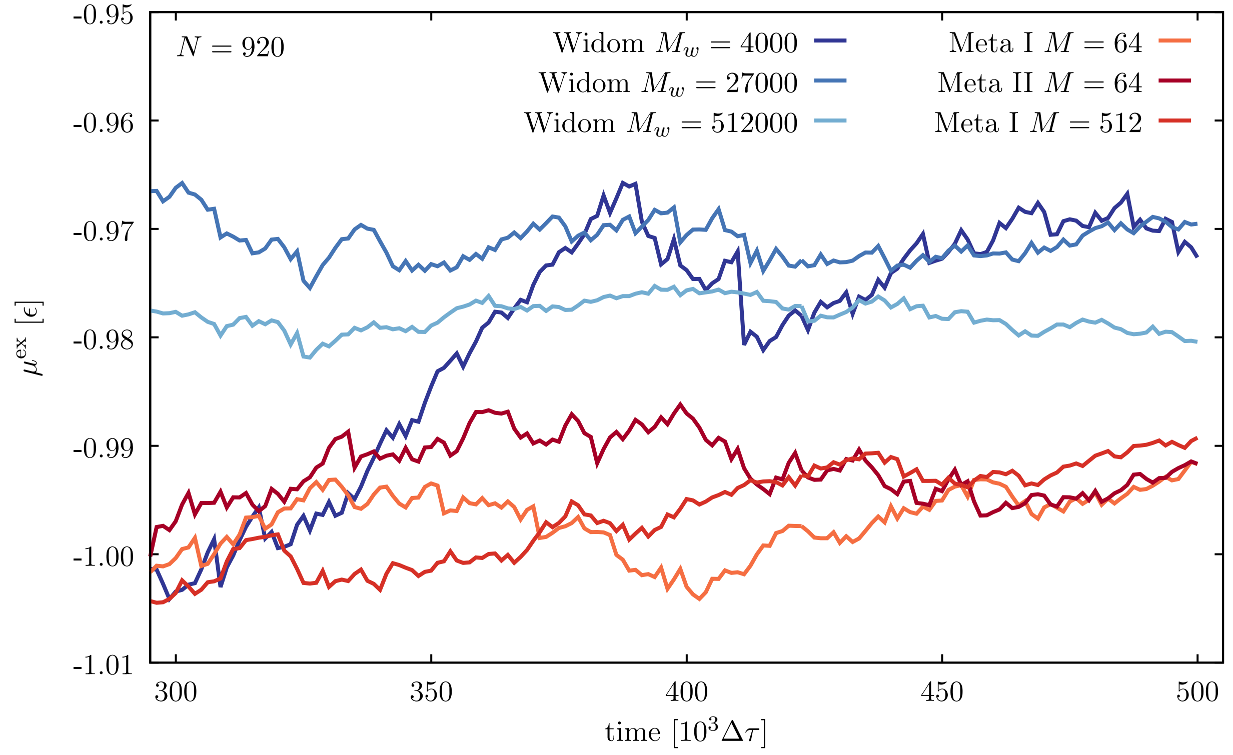


FIG. 1. $\mu^{ex}$ as a function of the MD time for the $N = 920$ system. The Widom calculation $M_w = 4000, 27000$ and $512000$ are compared to metadynamics results with $M = 64$ of type I and II and with $M = 512$ of type I (colors indicated in the legend). The final results, and respective statistical errors, are indicated in Tab. I.

## II. VARIATIONALLY ENHANCED SAMPLING

As mentioned in the main text, the sampling of $s$ in our technique can be driven using other biasing techniques than WT Metadynamics. In the following we present the results of employing the recently proposed Variationally Enhanced Sampling (VES) method[1]. In Sec. II A we provide a brief outline of the VES method, then, in Sec. II B, the choice of the target probability distribution is discussed. Finally, in Sec. II C, the results of VES calculations are reported.

## A. Introduction to VES

VES constructs a bias $V(s)$ by minimizing the following functional:

$$\Omega[V] = \beta^{-1} \frac{\int \mathrm{d}s\, \mathrm{e}^{-\beta[F(s)+V(s)]}}{\int \mathrm{d}s\, \mathrm{e}^{-\beta[F(s)]}} + \int \mathrm{d}s\, p_{\mathrm{t}}(s) V(s), \tag{1}$$

in which $F(s)$ is the free energy surface associated to the CV space and $p_{\mathrm{t}}(s)$ is a target probability distribution. As shown in Ref. 1, $\Omega[V]$ is convex, and its global minimum is given by:

$$V(s) = -F(s) - \beta^{-1} \log p_{\mathrm{t}}(s). \tag{2}$$

Thus, when the functional is minimized, the resulting $V(s)$ leads to a sampling according to the target distribution $p_{\mathrm{t}}(s)$. A possible approach to perform the minimization of $\Omega$ is to consider linear expansions for the bias potential:

$$V(s;\alpha) = \sum_k \alpha_k f_k(s), \tag{3}$$

where the $f_k(s)$ represent an appropriate basis set in the CV space. The $\alpha_k$ coefficients are optimized on-the-fly, using average stochastic gradient descent[2], so that $\Omega$ is minimized. The possibility of choosing a target sampling distribution $p_{\mathrm{t}}(s)$ represents a very useful feature for improving the efficiency of our calculations, as it will be shown in the following.

## B. Definition of the Target Probability Distribution

In this section we discuss the definition of the target distribution $p_{\mathrm{t}}$, used in the VES calculation of $\mu^{\mathrm{ex}}$ presented in Sec. II C. As mentioned in the main text, the calculation of $\mu^{\mathrm{ex}}$ requires accurate sampling of the negative $s^{\mathrm{r}}$ distribution tail. However also the sampling of the $p(s^{\mathrm{r}})$ main peak, which is located at higher values, is important to correctly estimate the statistical weights of the biased configurations[3].

To meet these sampling requirements, we define $p_{\mathrm{t}}$ as the sum of two Generalized Normal Distributions (GND). The GND family is a well-known generalization of the normal distribution, in which a shape parameter $\beta$ regulates the weight of the tails according to:

$$G(s;\hat{s},\alpha,\beta) = \frac{\beta}{2\alpha\Gamma(1/\beta)} \exp\left[-\frac{|s-\hat{s}|^{\beta}}{\alpha^{\beta}}\right], \tag{4}$$

| | $\hat{s}$ | $\alpha$ | $\beta$ | $A_i$ |
|---|---|---|---|---|
| $G_1$ | 35 | 45 | 10 | 0.5 |
| $G_2$ | -7 | 7 | 10 | 0.5 |

TABLE II. $p_{\mathrm{t}}$ parameters for the VES calculation presented in the main text.

in which $\Gamma$ is the the gamma function. For $\beta = 2$ Eq. 4 gives a Gaussian distribution with mean $\hat{s}$ and variance $\alpha^2/2$. As $\beta$ is increased, the distribution becomes more uniform in $s \in (\hat{s} - \alpha, \hat{s} + \alpha)$, while the importance of its tails is reduced. $p_{\mathrm{t}}$ defined is thus defined as:

$$p_{\mathrm{t}}(s^{\mathrm{r}}) = \left[A_1 G_1(s^{\mathrm{r}}) + A_2 G_2(s^{\mathrm{r}})\right], \tag{5}$$

where $G_1$ is a broad GND, which drives the sampling over the whole domain of the canonical $p(s^{\mathrm{r}})$, while $G_2$ is a tighter GND, focused on the $s^{\mathrm{r}} < 0$ region. The coefficients $A_i$, with $i = 1, 2$, set the relative weight of the two GNDs, and they are chosen so that $p_{\mathrm{t}}$ is normalized, that is $A_1 + A_2 = 1$.

We choose the $A_i$ coefficients, and the parameters of the $G_i$ as follows. First we have assigned equal weights $A_i = 0.5$, such that the rate of probability amplitudes for the two GNDs depends only on the respective width $\alpha$ and, to a minor extent, on the shape parameter $\beta$. Regarding the latter, we have chosen $\beta = 10$ for both $G_1$ and $G_2$, which determines two approximately uniform distributions for $s \in (\hat{s} - \alpha, \hat{s} + \alpha)$ and strongly damped elsewhere.

In order to appropriately choose $\hat{s}$ and $\alpha$ for the two $G_i$'s we perform a short, preliminary WT metadynamics run, that does not add a significant computational cost to our calculation. In Fig. 2 we compare the probability distributions resulting from a $500\,\Delta\tau$ WT metadynamics run with those of a long production run. The figure shows that this short simulation time is already sufficient to assess the limits of the target distribution. From Fig. 2 it is evident that the chosen $p_{\mathrm{t}}$ extends beyond the minimum $s_{\mathrm{min}}$ of the visited $s^{\mathrm{r}}$ region. Indeed, there is no need to set a boundary to the sampling in that region, since there is a very steep free energy barrier that will confine the sampling. This physical limit is given by the maximum number of LJ atoms that can surround an inserted particle, attractively interacting with it. The existence of this lower boundary suggests that the preliminary run is needed only to assess the "high energy" sampling limit. The chosen parameters are reported in Tab. II, while the resulting $p_{\mathrm{t}}$ distribution is shown in Fig. 2.

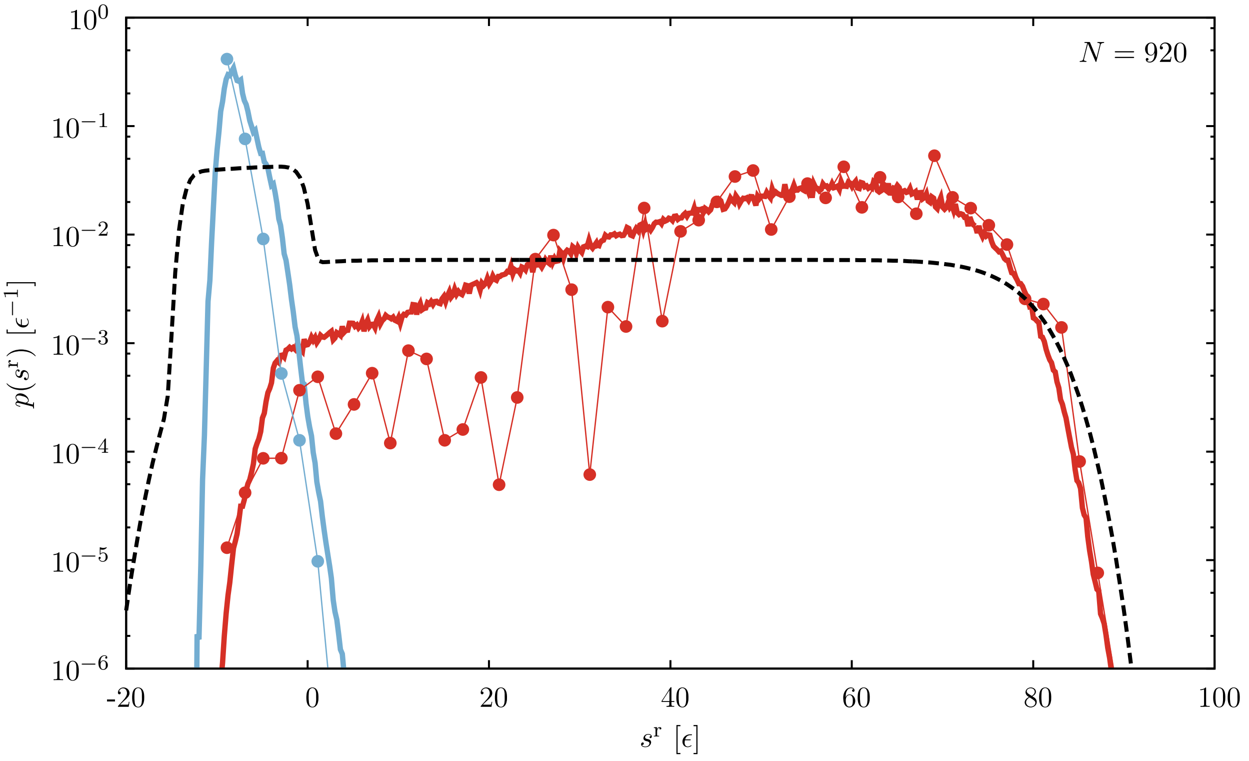


FIG. 2. Comparison of probability distributions of $s^{\mathrm{r}}$ ($M = 64$), obtained via a metadynamics simulation of the $N = 920$ system. We display the canonical probability $p(s^{\mathrm{r}})$ (red), and $p(s^{\mathrm{r}})\exp(-\beta s^{\mathrm{r}})$ (light blue curve). The thick lines correspond to the results after a running time of $1.5 \times 10^5\,\Delta\tau$, while the thin lines with dot markers represent the early results, after $500\,\Delta\tau$. The black dashed line indicates the $p_{\mathrm{t}}(s^{\mathrm{r}})$ of the VES calculations.

## C. VES results

We now show that the convergence of metadynamics results can be improved by applying the VES[1] method to enhance the sampling of $p(s^{\mathrm{r}})$. We recall that $s^{\mathrm{r}}$ is the regularized CV which is biased during the enhanced sampling run. It differs from $s$, that contains the full interaction potential. Since $s^{\mathrm{r}}$ is the driving CV, the VES target distribution controls its sampling, rather than that of $s$. However, as shown by the results reported in the following, the improved sampling of $p(s^{\mathrm{r}})$ is reflected on $p(s)$ as well.

We perform a VES simulation of the $N = 920$ system, and compare the result with the type I metadynamics run, discussed in the main text. For a rigorous comparison we use the same $M = 64$ insertion points of metadynamics calculation. As basis set for the bias

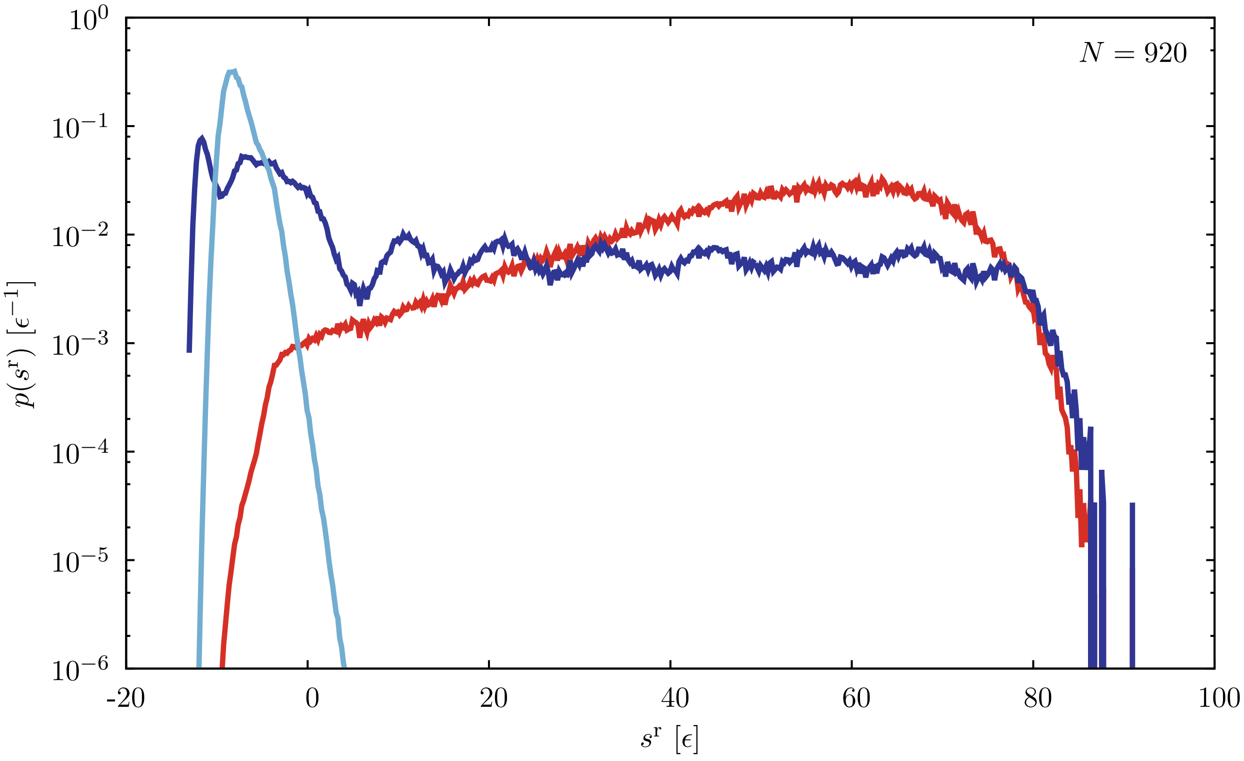


FIG. 3. Comparison of probabilty distributions of $s^{\mathrm{r}}$ ($M = 64$), obtained via a VES simulation of the $N = 920$ system. We display the canonical probability $p(s^{\mathrm{r}})$ (red curve), the biased ensemble probability $p_V(s^{\mathrm{r}})$ (blue curve) and $p(s^{\mathrm{r}})\exp(-\beta s^{\mathrm{r}})$ (light blue curve).

potential representation (see Eq. 3) we employ Legendre polynomials[4] up to the $32^{\mathrm{nd}}$ order, and the $\alpha_k$ coefficients are updated every $\Delta\tau = 500\Delta t$ (the same as the bias deposition time in the metadynamics run). The optimization step size used is $\mu = 0.1$ (for further details on the algorithm see Ref.[1]). As discussed in Sec. II B, the parameters of $p_{\mathrm{t}}$ are chosen building on a short, preliminary WT metadynamics sampling of $500\Delta\tau$.

In Fig. 3 we report the probability distributions obtained with the VES simulation. The biased probability distribution mimics the defined $p_{\mathrm{t}}$, focusing the sampling in the $s^{\mathrm{r}} < 0$ region. This higher sampling quality is reflected on the convergence of $\mu^{\mathrm{ex}}$. Indeed, in Fig. 4 we compare the convergence of $\mu^{\mathrm{ex}}$ resulting from the metadynamics and VES simulations, demostrating that the VES method is more efficient. The simulation time of VES results includes the $500\Delta\tau$ of WT metadynamics required for the definition of $p_{\mathrm{t}}$. We underline that the $\mu^{\mathrm{ex}}$ is computed using the $s$ variable, that is via reweighting procedure. This shows that the improvement in the sampling of $p(s^{\mathrm{r}})$ is conveniently reflected on $p(s)$.

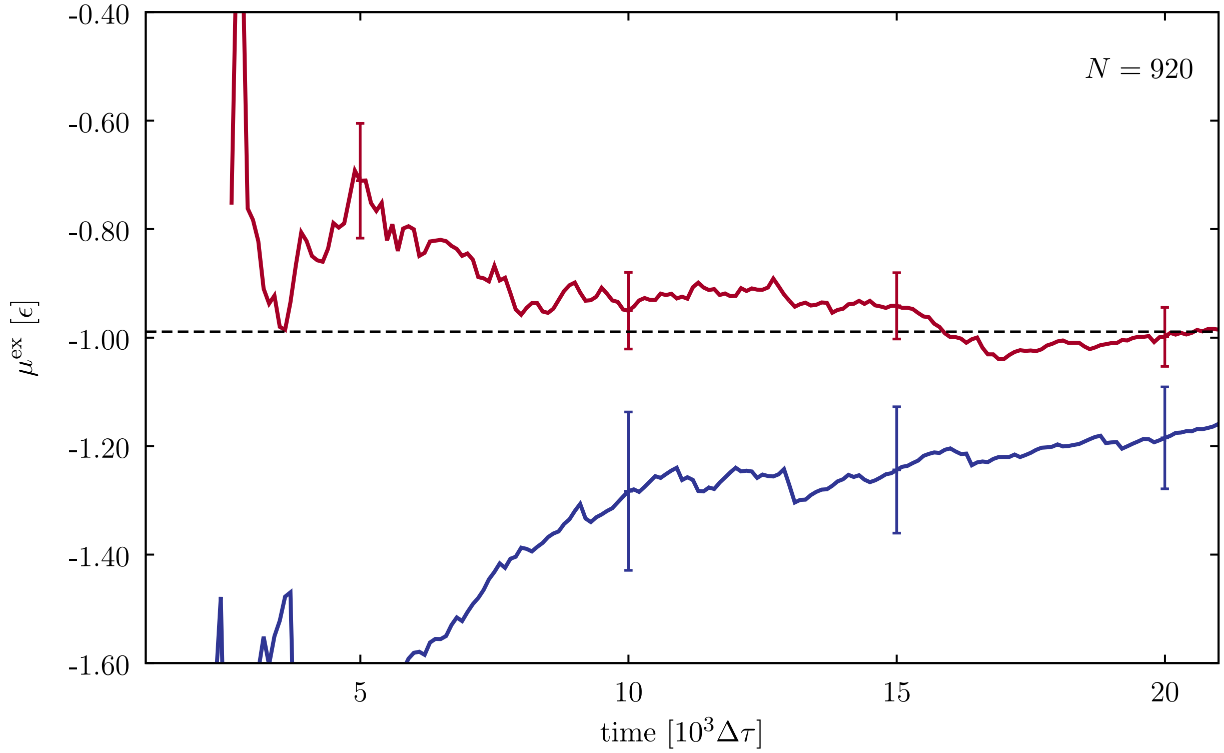


FIG. 4. $\mu^{\mathrm{ex}}$ as a function of the MD time for the $N = 920$ case. The result of a type I metadynamics calculation (blue curve) is compared to that of a VES calcultion (red curve), both performed with the same $M = 64$ insertion points. The black dashed line indicates a reference $\mu^{\mathrm{ex}}$ value obtained with a $M = 512$ metadynamics run of $5 \times 10^5 \Delta\tau$.

## REFERENCES


[1]O. Valsson and M. Parrinello, Phys. Rev. Lett. **113**, 090601 (2014).

[2]F. Bach and E. Moulines, in *Advances in Neural Information Processing Systems 26* (Curran, NY, 2013) pp. 773–781.

[3]O. Valsson, P. Tiwary, and M. Parrinello, Annual Review of Physical Chemistry **67**, 159 (2016), pMID: 26980304, http://dx.doi.org/10.1146/annurev-physchem-040215-112229.

[4]W. H. Press, S. A. Teukolsky, W. T. Vetterling, and B. P. Flannery, *Numerical Recipes 3rd Edition: The Art of Scientific Computing*, 3rd ed. (Cambridge University Press, New York, NY, USA, 2007).
